# Supplementary material for: Cross-view Geo-localization via Learning Disentangled Geometric Layout Correspondence
Source: arXiv:2212.04074 source file (2023-06-16)

Image id : 36267

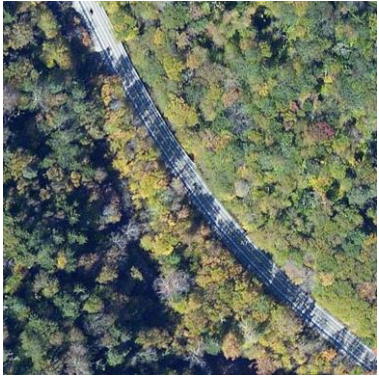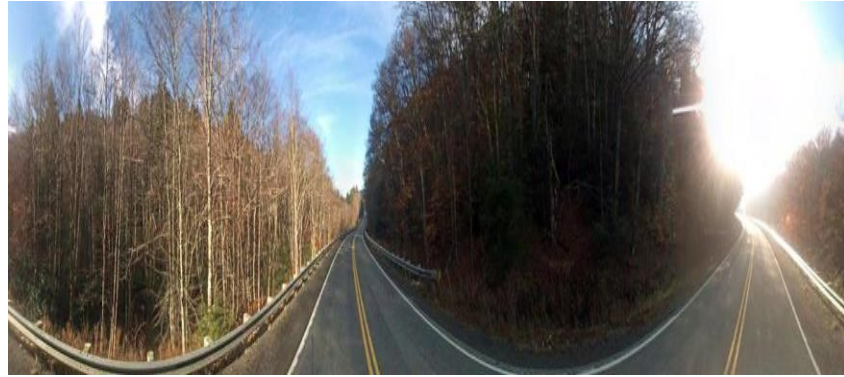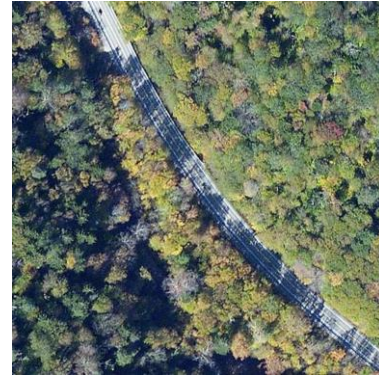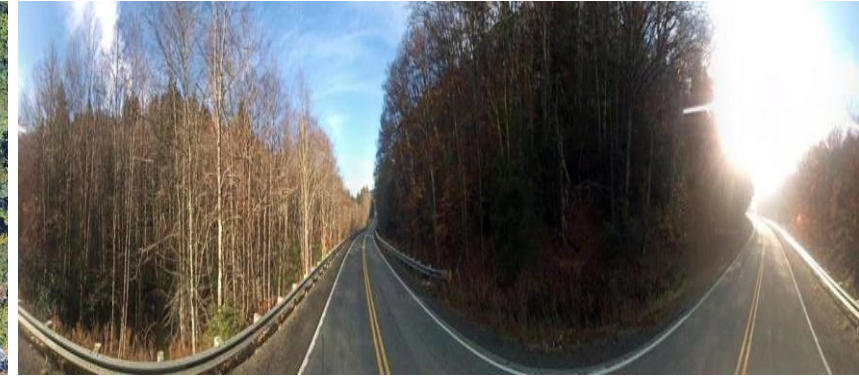

Image id : 15029

Image id : 11895

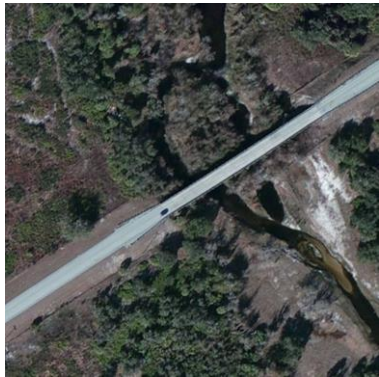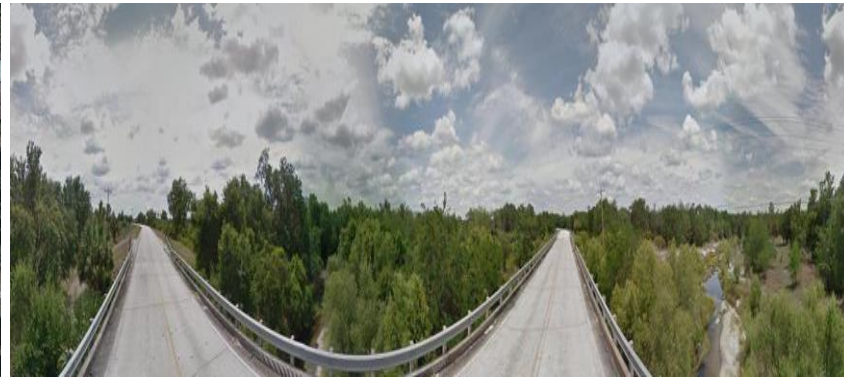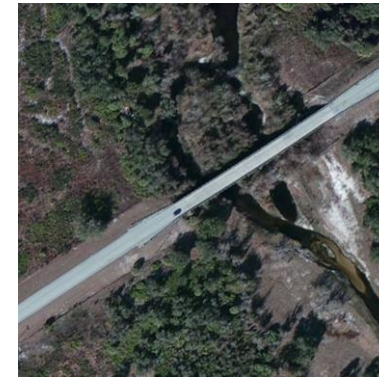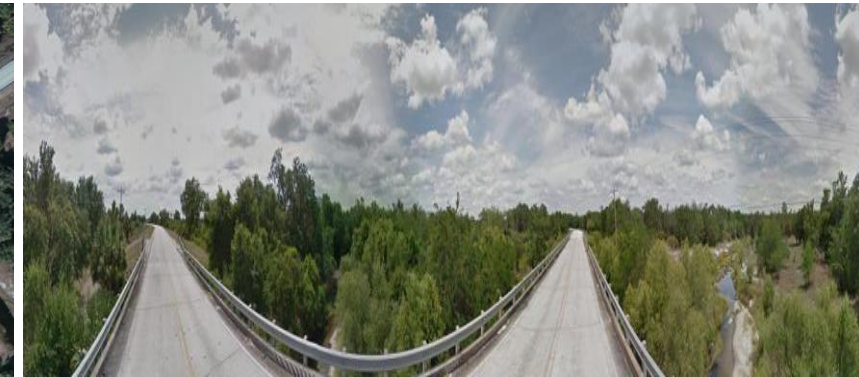

Image id : 15336

Image id : 23631

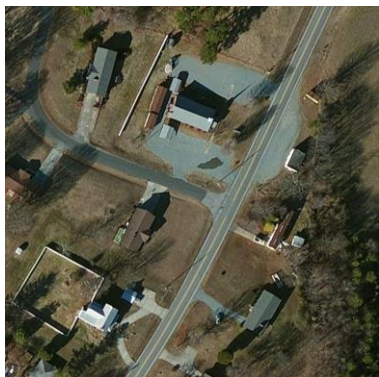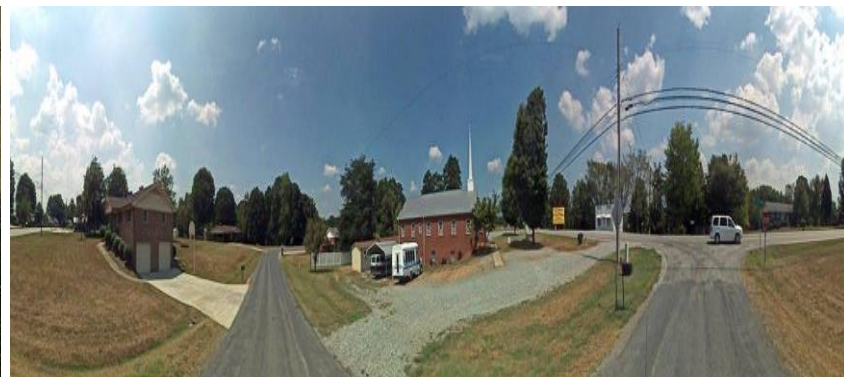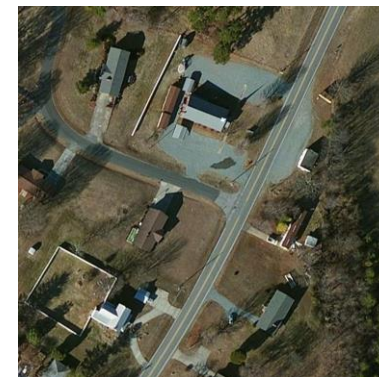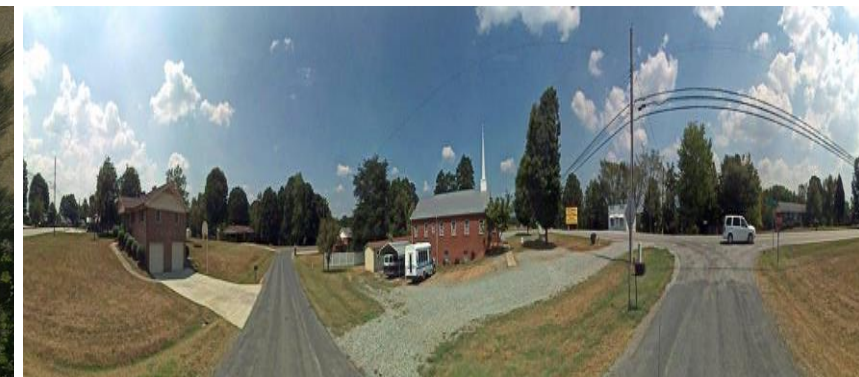

Image id : 24473



CVACT\_none\_none

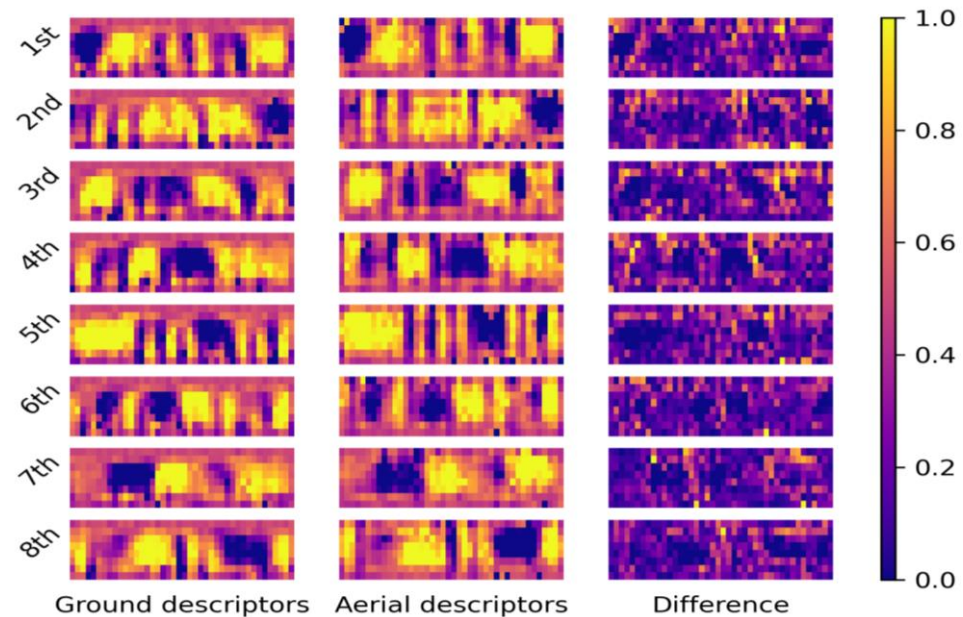

CVACT\_strong\_strong

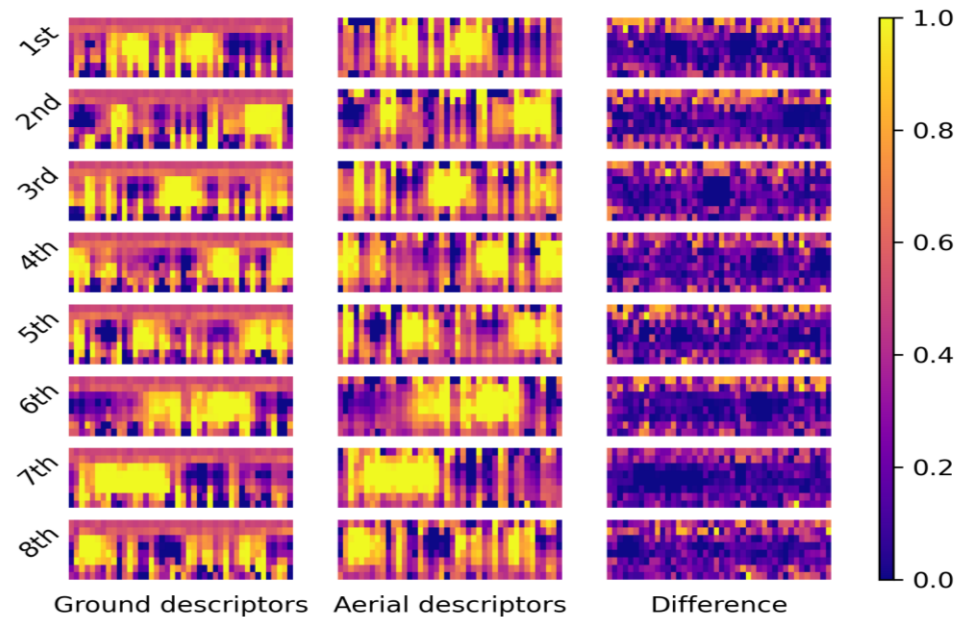

CVUSA\_none\_none

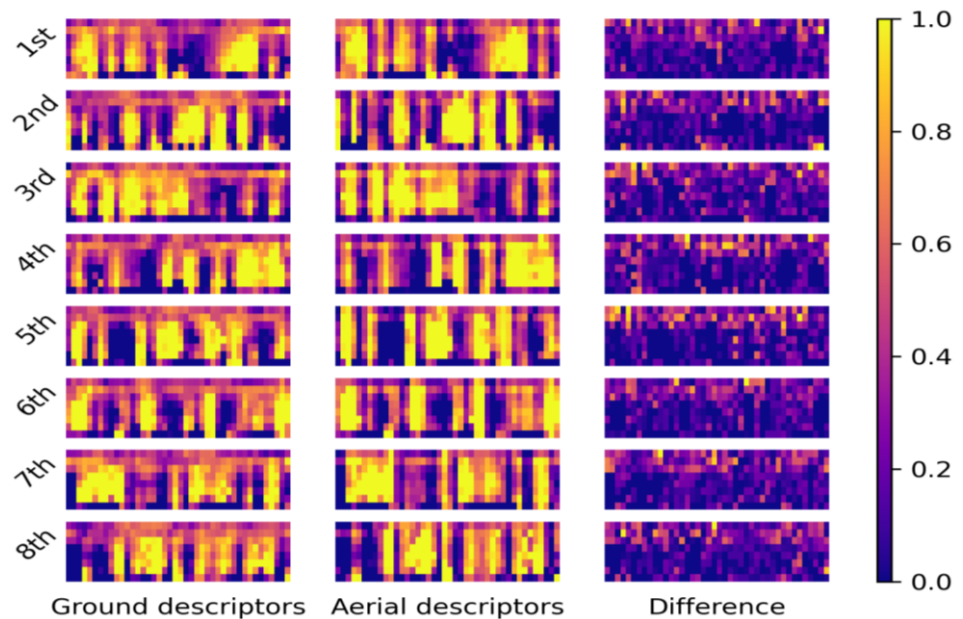

CVUSA\_strong\_strong

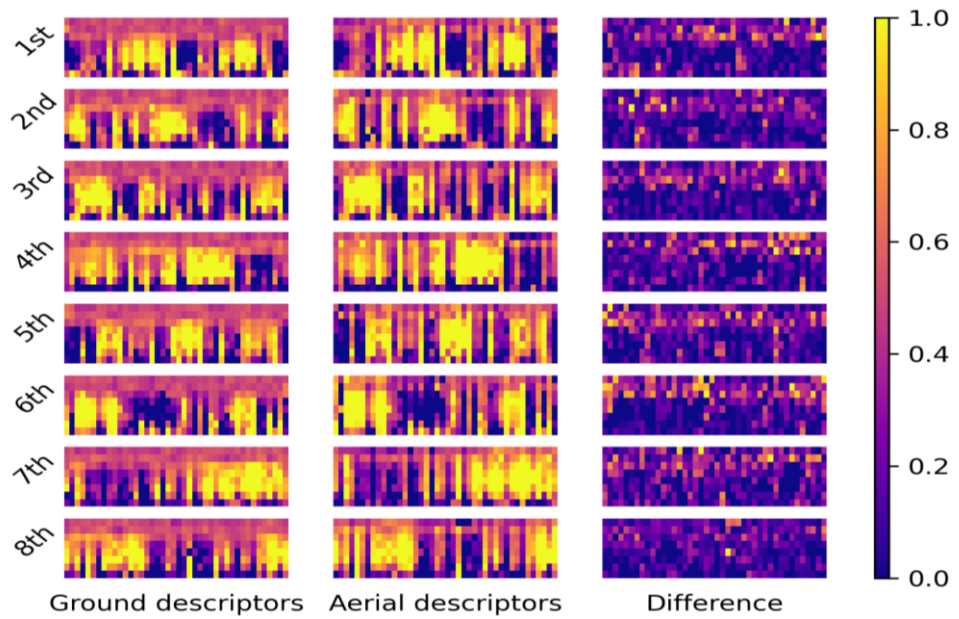

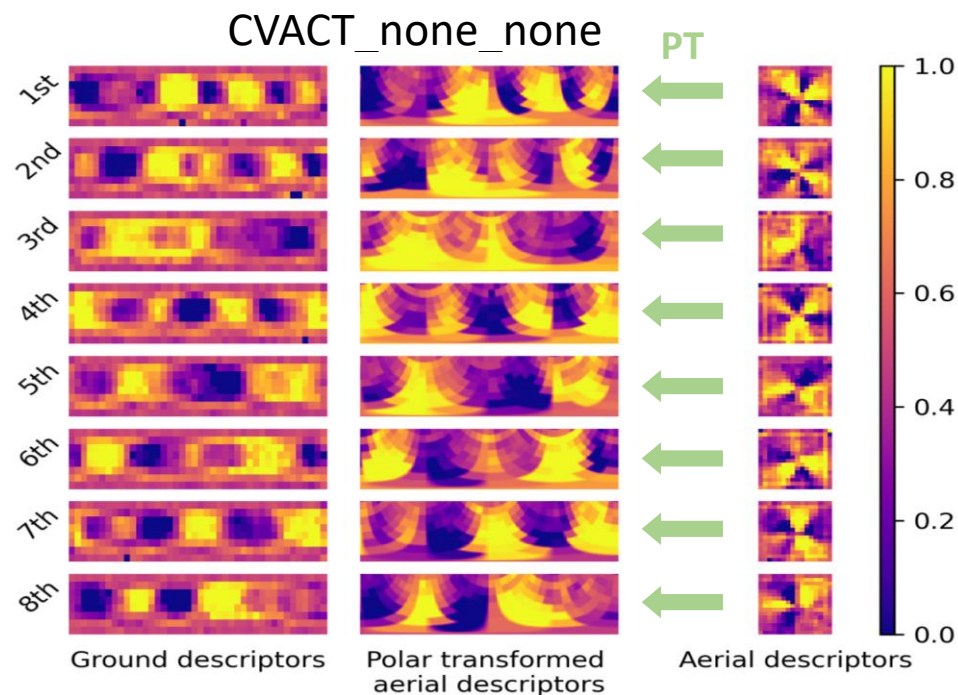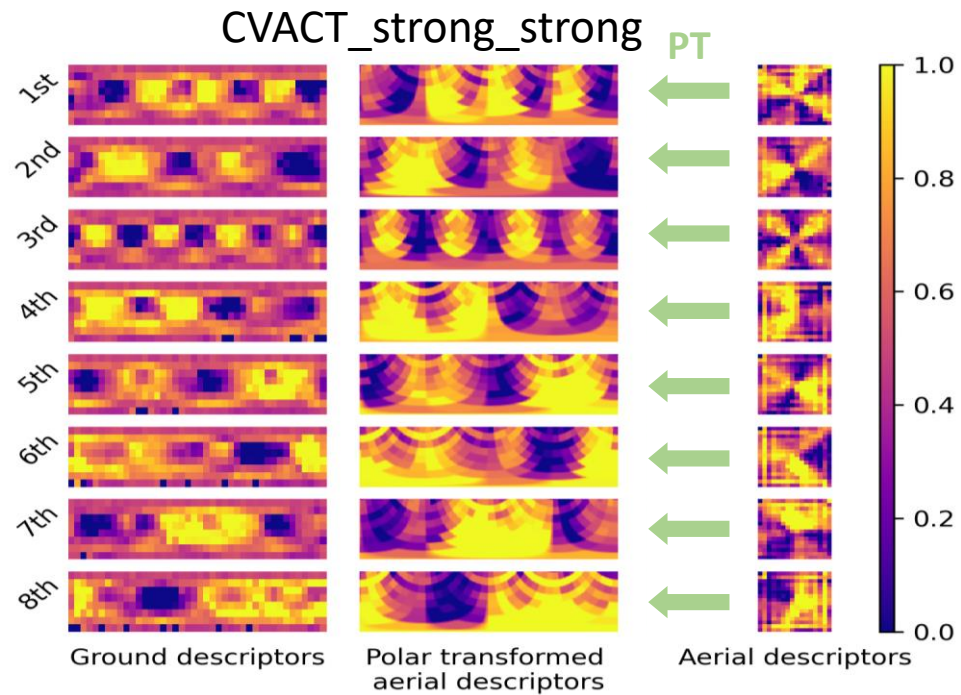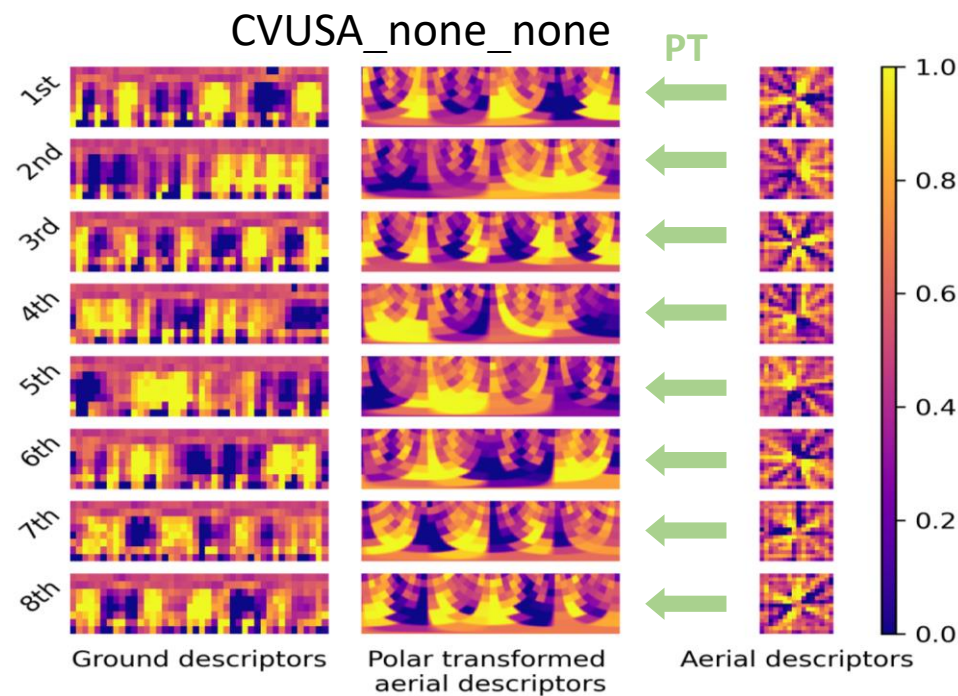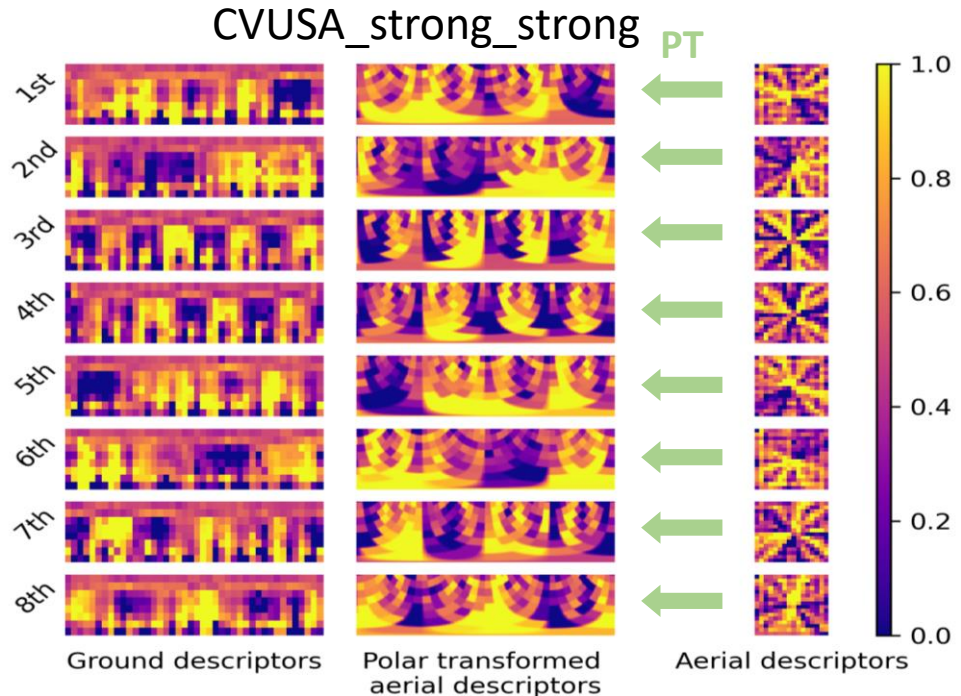

Supplement: Supplementary file 1 [file nips_supp.pdf]
